# Supplementary material for: Vector Projection Network for Few-shot Slot Tagging in Natural Language Understanding
Source: arXiv:2009.09568 source file (2020-09-22)
Supplement: Supplementary file 1 [file appendix.tex]

%
% File emnlp2020.tex
%
%% Based on the style files for ACL 2020, which were
%% Based on the style files for ACL 2018, NAACL 2018/19, which were
%% Based on the style files for ACL-2015, with some improvements
%%  taken from the NAACL-2016 style
%% Based on the style files for ACL-2014, which were, in turn,
%% based on ACL-2013, ACL-2012, ACL-2011, ACL-2010, ACL-IJCNLP-2009,
%% EACL-2009, IJCNLP-2008...
%% Based on the style files for EACL 2006 by 
%%e.agirre@ehu.es or Sergi.Balari@uab.es
%% and that of ACL 08 by Joakim Nivre and Noah Smith

\documentclass[11pt,a4paper]{article}
\usepackage[hyperref]{emnlp2020}
\usepackage{times}
\usepackage{latexsym}

\usepackage{amsmath}
\usepackage{amsfonts}
\usepackage{multirow,multicol}
\usepackage{pifont}
\usepackage{graphicx}

% This is not strictly necessary, and may be commented out,
% but it will improve the layout of the manuscript,
% and will typically save some space.
\usepackage{microtype}

%\aclfinalcopy % Uncomment this line for the final submission
%\def\aclpaperid{3340} %  Enter the acl Paper ID here

\setlength\titlebox{2.5cm}
% You can expand the titlebox if you need extra space
% to show all the authors. Please do not make the titlebox
% smaller than 5cm (the original size); we will check this
% in the camera-ready version and ask you to change it back.

\title{Appendix of Vector Projection Network for Few-shot Slot Tagging in Natural Language Understanding}

\begin{document}
\maketitle

\appendix

\input{app.tex}

\bibliography{emnlp2020} %anthology
\bibliographystyle{acl_natbib}

\end{document}
